# Supplementary material for: A survey on natural language processing (nlp) and applications in insurance
Source: arXiv:2010.00462 source file (2020-10-01)
Supplement: Supplementary file 1 [file appendix.tex]

\chapter{Your apprendix}

\section{Appendix section}

At the diagnosis, the stage of the cancer is assessed according to several features (size of tumor, extension, lymph nodes, ...). A breast cancer is a Carcinomas in Situ (CiS) when the tumour is confined to its original location and has not invaded the surrounding organs/tissues. Once the tumour is removed by a surgical practitioner, the patient is very likely to cure. The other stages have a worst prognosis. CiS are usually not covered by CI policies. All data recorded with a CiS behaviour are removed of the data set.
